# Supplementary material for: Setting the threshold for high throughput detectors: A mathematical approach for ensembles of dynamic, heterogeneous, probabilistic anomaly detectors
Source: arXiv:1710.09422 source file (2017-10-25)
Supplement: Supplementary file 1 [file 99-appendix.tex]

\section*{Appendix}
\addcontentsline{toc}{section}{Appendix}
\label{app:appendix}
